# Supplementary material for: Motif Prediction with Graph Neural Networks
Source: arXiv:2106.00761 source file (2022-05-21)
Supplement: Supplementary file 2 [file appendix-scores.tex]

\section*{Appendix G: Full Specification of Score Functions}

In this section we define the motif prediction score functions for Jaccard and Common Neighbors. In the correlated versions of these functions, we choose the weight vector $\mathbf{w}$ to assign the same importance to each link within the motif $M$. Moreover $\mathcal{E}$xisting edges each receive score~1. Notice that both the choice of $\mathbf{w}$ and of the score for $\mathcal{E}$xisting edges, can be determined directly by the user to incorporate domain knowledge for the motif of interest. 
 
\subsection*{Harnessing Jaccard}

We now provide full specifications of motif prediction score functions that
harness Jaccard scores for individual links.  Jaccard scores are normalized by
default, so we exclude any explicit normalization. 

\emph{No Positive Correlation, No Negative Correlation (Deal-Breaker Edges)}:

\begin{gather}
  \label{eq:jac_motif}
  s_{\perp}(M)^{J} = \prod_{e_{u,v} \in E_{M,\mathcal{N}}} \frac{\abs{N_u \cap N_v}}{\abs{N_u \cup N_v}} \prod_{e_{u,v} \in \overline{E}_{M,\mathcal{D}}} \left( 1 - {\frac{\abs{N_u \cap N_v}}{\abs{N_u \cup N_v}}}\right)
\end{gather}

\emph{Positive Correlation, No Negative Correlation (no Deal-Breaker Edges)}:

\begin{gather}
  \label{eq:cor_jac_motif}
  s(M)^{J} = \frac{1}{|E_{M}|} \;\; \left(\;\;  \sum_{e_{u,v} \in E_{M,\mathcal{N}}}^{} \frac{\abs{N_u \cap N_v}}{\abs{N_u \cup N_v}} + |E_{M,\mathcal{E}}|\;\; \right)
\end{gather}

\emph{Positive Correlation, Negative Correlation (Deal-Breaker Edges)}:

\begin{gather}
	\label{eq:cor_db_jac_motif}
	s^{*}(M)^{J} = \frac{1}{|E^{*}_{M}|} \;\; \left(\;\;  \sum_{e_{u,v} \in E_{M,\mathcal{N}}}^{} \frac{\abs{N_u \cap N_v}}{\abs{N_u \cup N_v}} \;\; - \sum_{e_{u,v} \in \overline{E}_{M,\mathcal{D},\mathcal{N}}}^{} \frac{\abs{N_u \cap N_v}}{\abs{N_u \cup N_v}}  + |E_{M,\mathcal{E}}| \;\; \right)
\end{gather}

where $E^{*}_{M} =
E_{M} \cup \overline{E}_{M,\mathcal{D}}$ is the
set of ``edges that matter for the score''. We also consider
$\overline{E}_{M,\mathcal{D},\mathcal{E}} = \emptyset$ to avoid the trivial
$s^{*}(M)^{J} = 0$ result.

\subsection*{Harnessing Common Neighbors Scores}

We also provide full specifications of motif prediction score functions that
harness Common Neighbors scores for individual links.

\emph{No Positive Correlation, No Negative Correlation (Deal-Breaker Edges)}:

\small
\begin{gather}
  \label{eq:cn_motif}
  s_{\perp}(M)^{CN} =  \prod_{e_{u,v} \in E_{M}} s(e_{u,v})  \prod_{e_{u,v} \in \overline{E}_{M,\mathcal{D}}} \left( 1 - s(e_{u,v}) \right)
\end{gather}
\normalsize

where $s(e_{u,v}) = \dfrac{\abs{N_u \cap N_v}}{\max_{e_{u,v} \in E^{*}_{M,\mathcal{N}}}(\abs{N_u \cap N_v})}$. This because for this specific scheme, $\ceil{\lVert \mathbf{s^{*}(e)} \rVert^{\infty}} =
\max_{e_{u,v} \in E^{*}_{M,\mathcal{N}}}(\abs{N_u \cap N_v})$ where
$E^{*}_{M,\mathcal{N}} = E_{M,\mathcal{N}} \cup
\overline{E}_{M,\mathcal{D},\mathcal{N}}$ is the set of
``$\mathcal{N}$on-existing'' edges.

\emph{Positive Correlation, No Negative Correlation (no Deal-Breaker Edges)}:

\begin{gather}
	\label{eq:cor_cn_motif}
	s(M)^{CN} = \frac{1}{|E_{M}|} \;\; \left(\;\; \dfrac{\sum_{e_{u,v} \in E_{M,\mathcal{N}}}^{} \abs{N_u \cap N_v}}{\max_{e_{u,v} \in E_{M,\mathcal{N}}}(\abs{N_u \cap N_v})} + |E_{M,\mathcal{E}}|\;\; \right)
\end{gather}

\emph{Positive Correlation, Negative Correlation (Deal-Breaker Edges)}:
\begin{gather}
  \label{eq:cor_db_cn_motif}
  s^{*}(M)^{CN} = \frac{1}{|E^{*}_{M}|} \;\; \left(\;\; \dfrac{\sum_{e_{u,v} \in E_{M,\mathcal{N}}}^{} \abs{N_u \cap N_v} -  \sum_{e_{u,v} \in \overline{E}_{M,\mathcal{D},\mathcal{N}}}^{} \abs{N_u \cap N_v}}{\max_{e_{u,v} \in E^{*}_{M,\mathcal{N}}}(\abs{N_u \cap N_v})} + |E_{M,\mathcal{E}}|\;\; \right)
\end{gather}

where all the quantities has been defined previously for eq. (\ref{eq:cn_motif}). Here we also consider
$\overline{E}_{M,\mathcal{D},\mathcal{E}} = \emptyset$ to avoid the trivial
$s^{*}(M)^{CN}$ result. 

\if 0
$s^{*}(M)$ is a \emph{transformed} link prediction score, i.e., it is a
score that considers not only the $\mathcal{N}$on-existing and
$\mathcal{E}$xisting edges in $M$ but also $\mathcal{D}$eal-breaker edges.
Moreover, $s^{*}(M)$ is a proper generalization of the simple link prediction
score in Eq.~(\ref{eq:cor-s-simple}). Of course, a more general function
$f(\mathbf{s^{*}(e)})$ (e.g., a non-linear one) could also be implemented and the
normalization constant $\ceil{\lVert \mathbf{s^{*}(e)} \rVert^{\infty}}$ may
also be modeled as a normalization vector if existing edges are required to
have different weights (as for the $\mathcal{N}$on-existing ones, thanks to the
vector $\mathbf{w}$). Indeed, the transformed motif score provides a highly
flexible environment for the user who can adapt $s^{*}(M)$ to the specific
needs of his domain (e.g., where a particular motif might arise more frequently
or with a predefined link importance within the motif).
\fi
